# Supplementary material for: Dynamical birefringence: Electron-hole recollisions as probes of Berry curvature
Source: arXiv:1706.08449 ancillary file (2017-10-12)
Supplement: Supplementary file 1 [file SI_Band_model.pdf]

# Electron-hole recollisions as probes of Berry curvature
# Supplementary: Band model

Qile Wu

September 13, 2017

Bulk GaAs is a direct gap zincblende semiconductor whose low-energy electronic properties are usually described by the six-band Kane model [1], which can be written as:

$$H = \begin{bmatrix} T & 0 & -\frac{1}{\sqrt{2}}Pk_+ & \sqrt{\frac{2}{3}}Pk_z & \frac{1}{\sqrt{6}}Pk_- & 0 \\ 0 & T & 0 & -\frac{1}{\sqrt{6}}Pk_+ & \sqrt{\frac{2}{3}}Pk_z & \frac{1}{\sqrt{2}}Pk_- \\ -\frac{1}{\sqrt{2}}k_-P & 0 & U+V & -\bar{S}_- & R & 0 \\ \sqrt{\frac{2}{3}}k_zP & -\frac{1}{\sqrt{6}}k_-P & -\bar{S}_-^\dagger & U-V & 0 & R \\ \frac{1}{\sqrt{6}}k_+P & \sqrt{\frac{2}{3}}k_zP & R^\dagger & 0 & U-V & \bar{S}_+^\dagger \\ 0 & \frac{1}{\sqrt{2}}k_+P & 0 & R^\dagger & \bar{S}_+ & U+V \end{bmatrix}, \quad (1)$$

where $T = E_c + \frac{\hbar^2}{2m_0}[(2F+1)k_\parallel^2 + (2F+1)k_z^2]$, $U = E_v - \frac{\hbar^2}{2m_0}(\gamma_1 k_\parallel^2 + \gamma_1 k_z^2)$, $V = -\frac{\hbar^2}{2m_0}(\gamma_2 k_\parallel^2 - 2\gamma_2 k_z^2)$, $\bar{S}_\pm = -\frac{\hbar^2}{m_0}\sqrt{3}k_\pm \gamma_3 k_z$, $R = -\frac{\hbar^2}{2m_0}(\sqrt{3}\mu k_+^2 - \sqrt{3}\bar{\gamma} k_-^2)$. $E_c$ and $E_v$ are respectively the band-edge of conduction bands and valence bands. $m_0$ is the free electron mass. $P, F, \gamma_1, \gamma_2, \gamma_3$ are parameters fitting to data from experiments, and $\mu = \frac{\gamma_3 - \gamma_2}{2}$, $\bar{\gamma} = \frac{\gamma_3+\gamma_2}{2}$, $\mathbf{k}_\parallel = (k_x, k_y)$, with $k_x$-, $k_y$-, and $k_z$-axis lying along [010], [001], [100] of the conventional cubic unit cell. The following is the basis used:

$$|u_1\rangle = |S\uparrow\rangle, |u_2\rangle = |S\downarrow\rangle, \quad (2)$$

$$|u_3\rangle = -\frac{1}{\sqrt{2}}|(X+iY)\uparrow\rangle, |u_4\rangle = -\frac{1}{\sqrt{6}}[|(X+iY)\downarrow\rangle - 2|Z\uparrow\rangle] \quad (3)$$

$$|u_5\rangle = \frac{1}{\sqrt{6}}[|(X-iY)\uparrow\rangle + 2|Z\downarrow\rangle], |u_6\rangle = \frac{1}{\sqrt{2}}|(X-iY)\downarrow\rangle \quad (4)$$

where $|S\rangle$ belongs to the irreducible representation $\Gamma_1$ of $T_d$ symmetry group, $|X\rangle, |Y\rangle, |Z\rangle$ belong to $\Gamma_4$, and $|\uparrow\rangle, |\downarrow\rangle$ are eigenvectors of the Pauli matrix $\sigma_z$ in spin space. The states $|u_1\rangle, |u_2\rangle$ are usually called electron components,

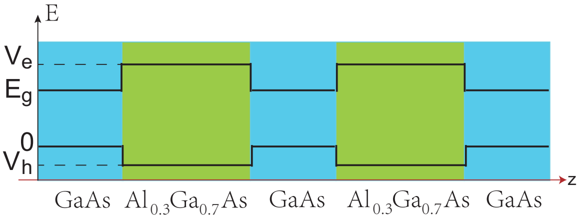


Figure 1: $GaAs/Al_{0.3}Ga_{0.7}As$ quantum well growing along [100]. The valence band edge of bulk $GaAs$ is taken to be zero, and $E_g$ is the bulk band gap. $V_e, V_h$ are the conduction band and valence band edges of the bulk $Al_{0.3}Ga_{0.7}As$.

$|E\rangle$. The states $|u_3\rangle, |u_4\rangle, |u_5\rangle, |u_6\rangle$ can also be labeled by the quantum number of spin-$\frac{3}{2}$. The states $u_3 = |\frac{3}{2}, +\frac{3}{2}\rangle$, $u_6 = |\frac{3}{2}, -\frac{3}{2}\rangle$ are usually called heavy-hole components denoted by $|HH\rangle$, while the states $u_4 = |\frac{3}{2}, +\frac{1}{2}\rangle$, $u_5 = |\frac{3}{2}, -\frac{1}{2}\rangle$ are the so-called light-hole components denoted by $|LH\rangle$. In bulk GaAs, the energy gap is about $1.55eV$ [2], so we neglect the coupling between electron and hole components and rewrite the matrix element $T$ as $E_c + \frac{\hbar^2}{2m_c^*}(k_\parallel^2 + k_z^2)$ with $m_c^*$ the effective mass of the bulk conduction band.

For the type-I quantum well growing along [100], as shown in Fig. 1, $k_x, k_y$ are still good quantum numbers. To calculate the band structure of the quantum well, we use the envelope function approximation [3], where $k_z$ is substituted by $-i\partial_z$ in the six-band Hamiltonian. To get a better behaved band structure for large momenta, the $\mathbf{k} \cdot \mathbf{p}$ Hamiltonian is extended to a tight-binding Hamiltonian for square lattice with lattice constant $\frac{\sqrt{2}}{2}a(a = 5.65\mathring{A}$ is the lattice constant of bulk GaAs), in which

$$T = E_c + \frac{\hbar^2}{2m_c^*}k_z^2 - (\frac{2}{a})^2\frac{\hbar^2}{m_c^*}[\cos(\frac{k_x a}{2})\cos(\frac{k_y a}{2}) - 1], \tag{5}$$

$$U+V = E_v - \frac{\hbar^2}{2m_0}(\gamma_1 - 2\gamma_2)k_z^2 + (\frac{2}{a})^2\frac{\hbar^2}{m_0}(\gamma_1+\gamma_2)[\cos(\frac{k_x a}{2})\cos(\frac{k_y a}{2}) - 1], \tag{6}$$

$$U-V = E_v - \frac{\hbar^2}{2m_0}(\gamma_1 + 2\gamma_2)k_z^2 + (\frac{2}{a})^2\frac{\hbar^2}{m_0}(\gamma_1-\gamma_2)[\cos(\frac{k_x a}{2})\cos(\frac{k_y a}{2}) - 1], \tag{7}$$

$$\bar{S}_\pm = -\frac{2\sqrt{3}\hbar^2}{m_0 a}\gamma_3[\sin(\frac{k_x a}{2})\cos(\frac{k_y a}{2}) \pm i\cos(\frac{k_x a}{2})\sin(\frac{k_y a}{2})]k_z, \tag{8}$$

$$R = \frac{4\sqrt{3}\hbar^2}{m_0 a^2}\{\frac{\gamma_2}{4}[\cos(k_y a) - \cos(k_x a)] - i\gamma_3\sin(\frac{k_x a}{2})\sin(\frac{k_y a}{2})\}. \tag{9}$$

In addition, we use the hard-wall approximation, assuming the height of the barrier is infinite. The effective well width used in the calculation is fitted to the positions of the exciton peaks in the absorption spectrum. How the parameters are chosen is described in the Appendix.

We first solve the eigenvalue problem at $\mathbf{k}_{\|} = \mathbf{0}$, where the six-band Hamiltonian is diagonal, from which we can get envelope functions of standing-wave forms with real space representation:

$$f_n(z) = \sqrt{\frac{2}{L}} \begin{cases} \cos(\frac{2m-1}{L}\pi z), & n = 2m-1 \\ \sin(\frac{2m}{L}\pi z), & n = 2m \end{cases}, \tag{10}$$

where $m = 1, 2, ...$, and $L$ is the effective well width. $f_n(z)$ is odd as a function of $z$ when $n$ is even, and even otherwise. As shown in the Appendix, the effective well widths for the electron and hole are slightly different. For simplicity, we neglect this difference in the calculation of the dipole matrix elements. So we will use the same symbol $f_n$ for the electron and hole envelope functions. For finite $|\mathbf{k}|$, HH and LH with the same envelope function couple through the matrix element $R$, and HH is mixed with LH through $\bar{S}_{\pm}$ if the parities of the envelope functions are different:

$$\int_{-L/2}^{L/2} f_n(z) f_m(z) dz = \delta_{m,n}, \tag{11}$$

$$\int_{-L/2}^{L/2} f_n(z)\partial_z f_m(z) dz = \frac{1}{L}\frac{4mn}{m^2-n^2}(-1)^{\frac{m+n+1}{2}}, mod(m-n,2) \neq 0. \tag{12}$$

Combining the six cellular functions $|u_j\rangle$ with the envelope functions $f_n(z)$, we get a basis for the quantum well, which are denoted as $|E_{n,\uparrow}\rangle = f_n|u_1\rangle$, $|E_{n,\downarrow}\rangle = f_n|u_2\rangle$ for the electron components, and $|HH_{n,\uparrow}\rangle = f_n|u_3\rangle$, $|HH_{n,\downarrow}\rangle = f_n|u_6\rangle$, $|LH_{n,\uparrow}\rangle = f_n|u_5\rangle$, and $|LH_{n,\downarrow}\rangle = f_n|u_4\rangle$ for the hole components. Note that in our model, for finite $|\mathbf{k}|$, $HH_{2m,\uparrow}$ only couples with $HH_{2m-1,\downarrow}$, $LH_{2m-1,\downarrow}$, and $LH_{2m,\uparrow}$, while $HH_{2m-1,\uparrow}$ only couples with $HH_{2m,\downarrow}$, $LH_{2m,\downarrow}$, and $LH_{2m-1,\uparrow}$. We use $f_n$ with $n = 1, 2, ..., 6$ for the valence bands.

Fig. 2 shows the subbands of the 5nm GaAs quantum well along [100]. The energy levels plotted are limited by the barrier heights. The subbands are labeled by the cellular functions at $\mathbf{k} = \mathbf{0}$.

# Appendix

To calculate the subbands, we need Luttinger parameters $\gamma_1, \gamma_2, \gamma_3$. the conduction band effective mass $m_c^*$, the band gap of the bulk material $E_g$, and the effective well width $L_e, L_h$ for electron and hole respectively.

Table. 1 lists the Luttinger parameters and conduction band effective masses. The parameters for $Al_xGa_{1-x}As$ are obtained from linear interpolation from the data for GaAs and AlAs.

To determine the energy gap $E_g$ of bulk GaAs, we make use of the absorption spectrum from experiment (Table. 2). The energy gap of the quantum well without exciton effect is the summation of the exciton gap

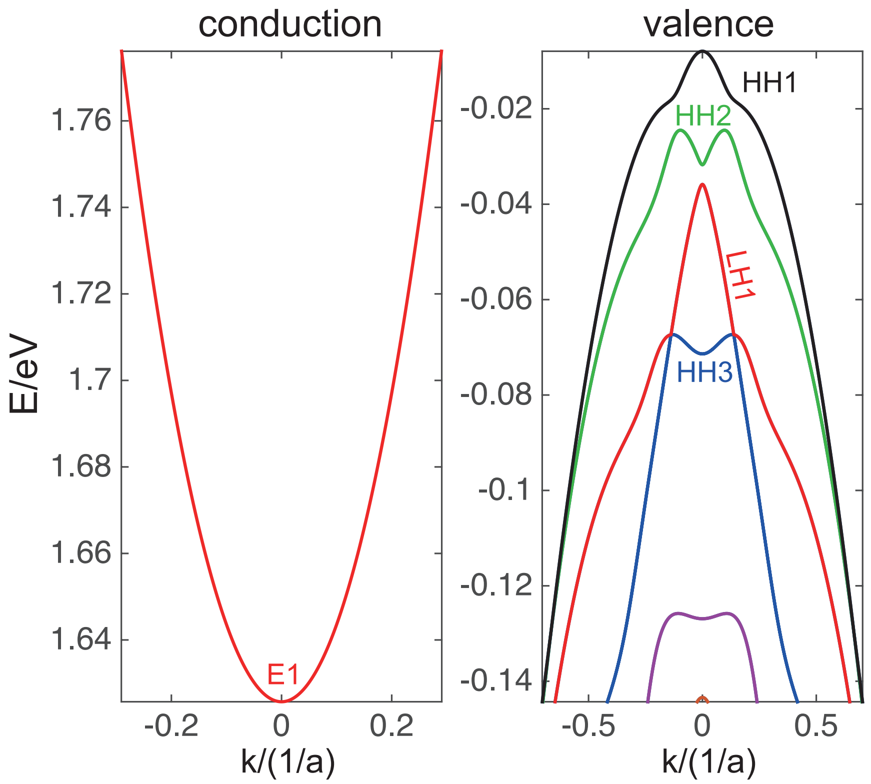


Figure 2: Subbands of the 5nm GaAs quantum well along [010].

| | $\gamma_1$ | $\gamma_2$ | $\gamma_3$ | $m_c^*/m_0$ |
|---|---|---|---|---|
| GaAs[2] | 6.9 | 2.2 | 2.9023 | 0.067 |
| AlAs[4] | 3.76 | 0.82 | 1.42 | 0.15 |
| $Al_{0.3}Ga_{0.7}As$ | 5.958 | 1.786 | 2.4576 | 0.091 |

Table 1: Luttinger parameters and conduction band effective masses. The parameters for $Al_xGa_{1-x}As$ are obtained from linear interpolation.

| | $\Delta_{HH-LH}/meV$ | $E_{xg}/eV$ |
|---|---|---|
| $10nm\ GaAs/Al_{0.3}Ga_{0.7}As$ | 10 | 1.552 |
| $5nm\ GaAs/Al_{0.3}Ga_{0.7}As$ | 25 | 1.620 |
| $10nm\ Al_{0.05}Ga_{0.95}As/Al_{0.3}Ga_{0.7}As$ | 10 | 1.620 |

Table 2: $\Delta_{HH-LH}$ is the exciton-splitting between E1-HH1 and E1-LH1. $E_{xg}$ is the E1-HH1 exciton gap.

|  | $\delta_{HH-LH}/meV$ | $E_q/eV$ | $L_h/nm$ | $L_e/nm$ | $E_g/eV$ |
|---|---|---|---|---|---|
| $10nm\ GaAs/Al_{0.3}Ga_{0.7}As$ | 13.1 | 1.5656 | 15.9 | 16.26 | 1.5406 |
| $5nm\ GaAs/Al_{0.3}Ga_{0.7}As$ | 28.1 | 1.6336 | 10.9 | 8.13 | 1.5406 |
| $10nm\ Al_{0.05}Ga_{0.95}As/Al_{0.3}Ga_{0.7}As$ | 13.2 | 1.6341 | 15.6 | 13.20 | 1.5993 |

Table 3: $\delta_{HH-LH}$ is the splitting between quantum well energy levels HH1 and LH1. $E_q$ is the energy gap of the quantum well.

$E_{xg}$ and the binding energy of the exciton, which reads in the Hydrogen-like atom model [5]

$$E_0 = \frac{2\mu e^4}{\hbar^2}(\frac{1}{4\pi\varepsilon_0\varepsilon})^2, \tag{13}$$

where $\mu$ is the reduced mass of the electron-hole pair, and $\varepsilon_0, \varepsilon$ are the vacuum dielectric constant and relative dielectric constant respectively. In the hard-wall approximation, we have

$$E_{E_1} = E_g + \frac{\hbar^2}{2m_0}\frac{m_0}{m_c^*}(\frac{\pi}{L_e})^2, \tag{14}$$

$$E_{HH1} = -(\gamma_1 - 2\gamma_2)\frac{\hbar^2}{2m_0}(\frac{\pi}{L_h})^2, \tag{15}$$

$$E_{LH1} = -(\gamma_1 + 2\gamma_2)\frac{\hbar^2}{2m_0}(\frac{\pi}{L_h})^2. \tag{16}$$

With the coupling between heavy hole and light hole neglected, the effective mass of HH1 and LH1 excitations are estimated as

$$m_{HH}^* = -\frac{m_0}{\gamma_1 + \gamma_2}, \tag{17}$$

$$m_{LH}^* = -\frac{m_0}{\gamma_1 - \gamma_2}. \tag{18}$$

From the Luttinger parameters listed above we obtain the reduced masses for the E1-HH1 and E1-LH1 electron-hole pairs $\mu_{ch} = 0.0416m_0$, $\mu_{cl} = 0.0510m_0$. Using $\varepsilon = 12.9$, we have the corresponding binding energies $E_{0,ch} = 13.6meV$, $E_{0,cl} = 16.7meV$. From these we can get the energy gap $E_q$, as well as the splitting of energy levels HH1 and LH1 without exciton effect, $\delta_{HH-LH}$(Table. 3). In this quantum well, usually the barrier is much higher for the electron than the one for the hole, so we assume that $L_e$ for the 10nm quantum well is twice of the one for the 5nm quantum well. For the hole, from $\delta_{HH-LH}$, $L_h$ can be calculated. $L_e$ and $E_g$ can be extracted from equation $E_{E_1} - E_{HH1} = E_q$. The values of $L_h, L_e, E_g$ are also listed in Table. 3.

The energy gap of $Al_xGa_{1-x}As$ is estimated here through empirical formula $E(x) = E_g + 1.155x + 0.37x^2$ [6]. Using the same dielectric constant $\varepsilon$,

the binding energies of the excitons in the $Al_{0.05}Ga_{0.95}As$ quantum well are estimated as $E_{0,ch} = 14.1meV$, $E_{0,cl} = 17.3meV$. The resulting parameters are listed in Table. 3.

For the height of the barrier, we assume that $V_e = 0.62[E(x) - E_g]$, $V_h = -0.38[E(x) - E_g]$ [6]. These values are used to determine the critical momenta at which the electron and hole reach the barrier region.

## References


[1] E O Kane. Band structure of indium antimonide. *Journal of Physics and Chemistry of Solids*, 1(4):249–261, 1957.

[2] M Cardona and Y Y Peter. *Fundamentals of semiconductors.* Springer, 2005.

[3] Lok C Lew Yan Voon and Morten Willatzen. *The kp method: electronic properties of semiconductors.* Springer Science & Business Media, 2009.

[4] I Vurgaftman, J R Meyer, and L R Ram-Mohan. Band parameters for iii–v compound semiconductors and their alloys. *Journal of applied physics*, 89(11):5815–5875, 2001.

[5] X L Yang, S H Guo, F T Chan, K W Wong, and W Y Ching. Analytic solution of a two-dimensional hydrogen atom. I. Nonrelativistic theory. *Physical Review A*, 43(3):1186, 1991.

[6] Miyoko Oku Watanabe, Jiro Yoshida, Masao Mashita, Takatosi Nakanisi, and Akimichi Hojo. Band discontinuity for GaAs/AlGaAs heterojunction determined by C-V profiling technique. *Journal of applied physics*, 57(12):5340–5344, 1985.
