# Supplementary material for: Dynamical birefringence: Electron-hole recollisions as probes of Berry curvature
Source: arXiv:1706.08449 ancillary file (2017-10-12)
Supplement: Supplementary file 2 [file SI_Experiment.pdf]

# Electron-hole recollisions as probes of Berry curvature

# Supplementary: Experiment

Hunter B. Banks,[1,2] Qile Wu,[3,4] Darren C. Valovcin,[1,2] Shawn Mack,[5]
Arthur C. Gossard,[6] Loren Pfeiffer,[7] Renbao Liu,[3] and Mark S. Sherwin[1,2]

[1]*Physics Department, University of California, Santa Barbara, USA*

[2]*Institute for Terahertz Science and Technology,*
*University of California, Santa Barbara, USA*

[3]*Department of Physics, The Chinese University of Hong Kong, Hong Kong, China*

[4]*Department of Physics, Tsinghua University,*
*Beijing 100084, People's Republic of China*

[5]*U.S. Naval Research Laboratory, Washington, DC, USA*

[6]*Materials Department, University of California, Santa Barbara, USA*

[7]*Electrical Engineering Department,*
*Princeton University, Princeton, NJ, USA*

(Dated: September 13, 2017)

| | 5 nm GaAs QWs | 10 nm AlGaAs QWs | 10 nm GaAs QWs | |
|---|---|---|---|---|
| | 50 nm GaAs | 50 nm GaAs | 150 nm GaAs | |
| | 40 nm $Al_{0.3}Ga_{0.7}As$ | 40 nm $Al_{0.3}Ga_{0.7}As$ | 50 nm $Al_{0.3}Ga_{0.7}As$ | |
| $N$ repeats | 20 nm $Al_{0.3}Ga_{0.7}As$ | 20 nm $Al_{0.3}Ga_{0.7}As$ | 15 nm $Al_{0.3}Ga_{0.7}As$ | |
| | 5 nm GaAs | 10 nm $Al_{0.05}Ga_{0.95}As$ | 10 nm GaAs | QW region |
| | 20 nm $Al_{0.3}Ga_{0.7}As$ | 20 nm $Al_{0.3}Ga_{0.7}As$ | 15 nm $Al_{0.3}Ga_{0.7}As$ | |
| | 40 nm $Al_{0.3}Ga_{0.7}As$ | 40 nm $Al_{0.3}Ga_{0.7}As$ | 50 nm $Al_{0.3}Ga_{0.7}As$ | |
| | 50 nm GaAs | 50 nm GaAs | 150 nm GaAs | |
| | 300 nm $Al_{0.7}Ga_{0.3}As$ | 300 nm $Al_{0.7}Ga_{0.3}As$ | 300 nm $Al_{0.735}Ga_{0.265}As$ | Etch stop |
| | 50 nm GaAs | 50 nm GaAs | 100 nm GaAs | |
| | 500 $\mu$m GaAs | 500 $\mu$m GaAs | 500 $\mu$m GaAs | Substrate |

TABLE S1: The molecular beam epitaxial growth of the three samples, the 5 nm GaAs QWs, the 10 nm AlGaAs QWs, then the 10 nm GaAs QWs on the right. All samples are symmetric above etch stop layer. The number of repeats is given by $N$, where $N = 20$ for the 5 nm GaAs QWs and the 10 nm AlGaAs QWs, and $N = 10$ for the 10 nm GaAs QWs. The 5% AlGaAs in the well region of the 10 nm AlGaAs QWs was grown digitally. The 10 nm GaAs QWs were grown at 612° C, with 10 second pauses after each 10 nm GaAs well region, and 100 second pauses after every other GaAs layer.

## SAMPLE GROWTH AND PROCESSING

Three quantum well (QW) samples with varying degrees of quantum confinement and quenched disorder were grown by molecular beam epitaxy, see Table S1. The 5 nm GaAs sample consists of twenty 5 nm GaAs QWs with 20 nm $Al_{0.3}Ga_{0.7}As$ barriers. The 10 nm AlGaAs sample consists of twenty 10 nm $Al_{0.05}Ga_{0.95}As$ QWs with 20 nm $Al_{0.3}Ga_{0.7}As$ barriers. The 10 nm GaAs sample consists of ten 10 nm GaAs QWs with 15 nm $Al_{0.3}Ga_{0.7}As$ barriers, grown with interrupts at AlGaAs-on-GaAs interfaces for very smooth walls [1–4]. All the samples were grown on (100) semi-insulating GaAs substrates.

The samples were processed to allow for optical transmission experiments and to passively increase the local THz field inside the QWs. The NIR-absorbing GaAs substrate was lapped and etched away and the resulting micron-thick film was Van der Waals-bonded to a sapphire

substrate. With a total thickness on the order of the THz wavelength, interference from the incident field and reflections off the back surface of the substrate affect the THz field strength at the front surface, in the QWs. This interference leads to a periodic dependence of the THz field strength on the THz frequency in the QWs, which is usually undesirable. We chose to enhance this interference by depositing a THz-reflective, optically-transparent film of indium-tin oxide (ITO) on back surface of the sapphrie substrate.

**Epitaxial layer transfer process**

We transferred the multiple quantum wells from the growth GaAs substrate to a c-plane (0001) sapphire substrate to do optical experiments in transmission. To perform the transfer, we used a process developed by Garrett Cole, *et al.*, of Crystalline Mirror Solutions [5, 6], building upon work done by Eli Yablonovitch [7, 8]. This process brings an exposed epitaxial ("epi") growth layer and a very clean sapphire wafer into contact. Because both surfaces are very clean and smooth, Van der Waals forces, which are spread across the entire millimeter-sized sample, are strong enough to bond the surfaces.

First, the wafer was cleaved into $4 \times 9$ mm pieces. The substrate of the samples was then lapped down from 500 microns to about 150 microns thick. To support the sample during the etching and bonding process, Apiezon W, or black wax, was melted onto the growth side of the thinned samples. To begin the etching, any residual oxide layer that might lead to uneven substrate etching was removed with a 30:1 $H_2O$:$NH_4OH$ for 30 seconds. The remaining GaAs substrate, up until the etch stop layer, was then etched away using a 30:1 30% $H_2O_2$:$NH_4OH$, which removes approximately 1.7 microns/minute. The etch stop layer is removed using a one to two minute dip in buffered HF. Once the substrate is entirely etched away, stress inside the black wax causes the epi layer to bulge out slightly, making contact during the bonding step much easier. The sapphire wafer is thoroughly cleaned in solvents, followed by a 100 W, 300 mtorr $O_2$ descum. To bring the two surfaces into contact, the epi layer was mounted facing upwards, and a small drop of water was dripped onto it. The sapphire was then carefully pressed into contact with the epi layer, and the expelled water was wicked away with a clean wipe. Once the first sapphire-GaAs contact is made, the bonding area will expand as the very thin layer of water evaporates away. To encourage evaporation, the samples are kept under rough vacuum overnight. Once the

water has evaporated away and the surfaces are bonded strongly, the black wax is dissolved away in chloroform. Because no extra materials are needed to create the bond, there are no confounding problems like strong terahertz absorption or stress-induced birefringence. GaAs and sapphire also have similar thermal expansion coefficients, so thermal cycling between 15 K and 294 K does not harm the sample.

**Indium-tin oxide deposition**

To create constructive interference of the incoming THz wave and the reflected wave off the back side of the sapphire, an indium-tin oxide (ITO) film was deposited using an electron beam deposition chamber. The sapphire was heated to approximately 290 °C during deposition in an atmosphere of $3 \cdot 10^{-4}$ mtorr $O_2$. The initial deposition rate was set at 0.01 nm/s. It was increased to 0.03 nm/s after the first 20 minutes of deposition and increased further to 0.05 nm/s after an additional 20 minutes. After depositing 300 nm of ITO, the substrate was cooled to 140 °C before venting to atmosphere. The complex index of refraction is $\tilde{n} = 1.8 + i4 \cdot 10^{-4}$ at 750 nm, measured by an ellipsometer. The very small complex component of the index means that there will be no appreciable optical absorption by the ITO. The sheet resistance of the film is 12.6 $\Omega/\square$, measured by a resistivity mapper.

**Measurement of terahertz field enhancement**

The field enhancement as a function of frequency, $\kappa(f_{\mathrm{THz}})$, was measured using a frequency-extended vector network analyzer (VNA) as a quasi-optical vector reflectometer [9, 10]. Schottky diode multipliers and dividers in the transmitter and receiver extend the 0–40 GHz frequency domain of the VNA to 70–700 GHz, and precision horns couple the light to and from free space. The reflectometer is set up so that a transmitter illuminates a planar sample. The reflected light is then split off by a beam splitter and directed towards a receiver. Because the reflectometer operates in the frequency domain, Fabry-Perot interferences develop that can confound the signal. By running a calibration routine through the VNA on a metal mirror, the phase changes from the beam path can be calibrated out. The reflection spectrum of the sapphire-ITO cavity then represents the electric field at the sapphire surface where the QWs will be. This measurement has been done both with and

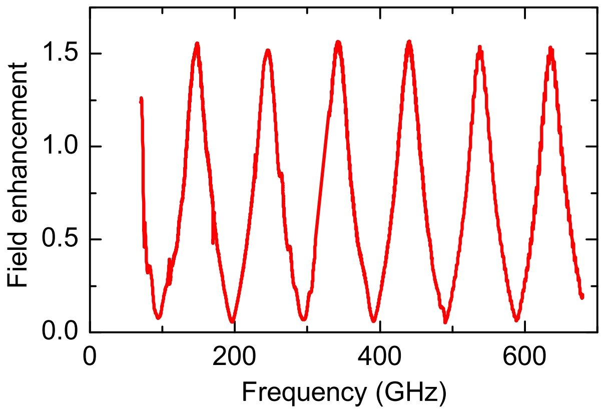


FIG. S1: The electric field enhancement multiplier as a function of THz frequency. The THz electric field is enhanced at the front surface of the sapphire due to interference of the incident and ITO-reflected THz fields. At the frequency used in the experiment, 540 GHz, the electric field is enhanced by 50%, and the intensity is more than two times stronger, a very significant increase for a nonlinear effect like HSG.

without QWs on the front surface, and there is little difference.

The large THz reflection off the film facilitates the interference at the front surface of the substrate, enhancing the electric field at certain frequencies inside the QWs by more than 50%, see Fig. S1, though some other frequencies suffer almost complete destructive interference. The free-electron laser (FEL) is broadly tunable in frequency with a very narrow linewidth, and HSG is not restricted by resonant effects from the THz field, so the THz frequency can be chosen solely based on the results of sample processing. The ITO film is transparent at NIR wavelengths, so it does not attenuate the NIR laser or the sidebands.

## OPTICAL METHODS

### Absorption measurement

The absorption spectra were measured by the differential transmission of a tungsten-halogen lamp, comparing the spectrum of the lamp transmitted through the sample and just through air. The sapphire substrate forms an NIR etalon, which adds a short-period sinusoid with an amplitude approximately 30% of the transmission signal, but is removed

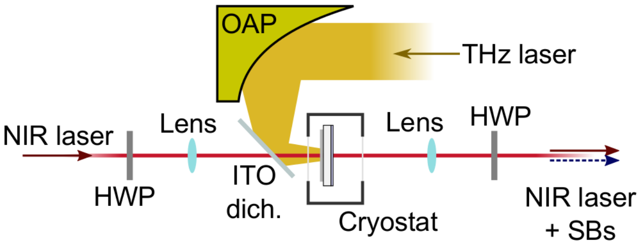


FIG. S2: Schematic of the optical setup. The direction of the linear polarization of the NIR laser is controlled by an achromatic half-wave plate (HWP) before the beam is focused onto the sample. The THz laser is focused with an off-axis parabolic mirror (OAP). The NIR and THz lasers are made copropagating with an ITO-coated glass slide as a dichroic mirror. The sample is held in a cryostat at 15 K. The NIR laser and sidebands (SBs) are collimated before the second achromatic HWP is rotated to the preferred direction of the detector.

in software using a short pass Fourier filter.

### Sideband measurement

Sidebands are generated by focusing the THz and NIR laser beams at the same spot on the sample with collinear propagation in the $[00\bar{1}]$ direction, see Fig. S2. The effective THz field strength in the QWs, $|\mathbf{F}_{\mathrm{THz}}|$, was kept at $35 \pm 2$ kV/cm for all experiments, and the THz frequency, $f_{\mathrm{THz}}$, was held at 540 GHz. The THz photon energy (2.23 meV) is far from resonance with the 1s-2p transition, avoiding complications from strong-field, nonlinear interactions [11]. The beam from the FEL was attenuated slightly to maintain a consistent field strength in the QWs using a pair of wire grid polarizers as a tunable attenuator. This strong THz field was generated using the cavity dump mode of the FEL, which produces a 40 ns-long THz pulse with a linewidth of less than 1 GHz [12]. The THz electric field is polarized horizontally for all experiments. The radius of the THz laser spot is 0.5 mm. The exciting NIR field comes from a continuous-wave MSquared SolsTiS-1200-PSX-XF Ti:sapphire laser. For both the 5 nm GaAs sample and the 10 nm AlGaAs sample, $\lambda_{\mathrm{NIR}} = 764$ nm (1.6227 eV), while for the 10 nm GaAs sample, $\lambda_{\mathrm{NIR}} = 798$ nm (1.5529 eV). The power of the NIR laser incident on the sample, $P_{\mathrm{NIR}}$, was held at 50 mW for all polarizations. The NIR power was

chosen to maximize the signal without overheating the samples. An achromatic half-wave plate rotated the NIR laser polarization between horizontal and vertical. The NIR and THz laser beams were made collinear with an ITO-coated glass slide at 45°, see Fig. S2. The radius of the NIR laser spot is approximately 100 $\mu$m. The lattice orientation was measured using a camera capable of imaging the sample while it is mounted in the cryostat. Cracks along cleavage planes indicated the lattice orientation. The samples, once mounted, were stationary, so rotations were performed by hand during mounting.

The sideband conversion efficiency is the power in the sideband divided by the power of the NIR laser incident on the sample, $P_{\text{SB}}/P_{\text{NIR}}$. The laser line and sidebands of order $n \leq 16$ were sent through a monochromator and measured by a photomultiplier tube (PMT). The strength of a sideband measured by the PMT is the integral of the sideband peak. The NIR laser itself was measured using the PMT to calibrate the optics and the detector so that the conversion efficiency for the low-order sidebands could be measured directly. The sidebands of order $n \geq 8$ were sent through an imaging spectrometer to an Andor NewtonEM CCD, which is capable of 5 minute exposures, capturing 300 FEL repetitions in a single image to minimize the readout noise. A short pass filter with a sharp cutoff from Semrock prevented the laser line from entering the spectrometer. The sidebands ($8 \leq n \leq 16$) that were measured by both the PMT and the CCD set the factor by which we scaled the highest order sideband strengths into the sideband conversion efficiencies. The strength of a sideband measured by the CCD is the area of a Gaussian fit to the sideband peak.

**Optical polarization measurement**

Measuring the complete polarization state of the sidebands is straightforward in the optical regime. The full set of Stokes parameters for each sideband was measured using a homemade Stokes polarimeter (see [13]). The four Stokes parameters are defined as follows:

$$S_0 = I$$
$$S_1 = pI \cos 2\alpha \cos 2\gamma$$
$$S_2 = pI \sin 2\alpha \cos 2\gamma$$
$$S_3 = pI \sin 2\gamma,$$

where $I$ is the intensity of the light, $p\,(\in [0,1])$ is the degree of polarization, $\alpha\,(\in [0,\pi])$ is the angle of the major axis of the polarization ellipse, and $\gamma\,(\in [-\pi/4,\pi/4])$ is the ellipticity of the polarization ellipse, see Fig. S4(a). For example, $(\alpha,\gamma)$ of horizontal light would be $(0,0)$, vertical $(\pi/2,0)$, and right circular light $(0,\pi/4)$. The Stokes polarimeter was built using an achromatic quarter wave plate (QWP) mounted on a rotation stage that was placed immediately behind the exit window of the cryostat, and a polarizer oriented perpendicular to the incident NIR laser polarization that was placed immediately behind the QWP, see Fig. S4(a). Fixing the polarization directly behind the cryostat prevented complications from the wavelength-dependent retardance of the dielectric mirrors or any polarization dependence of the detector. Let us define the QWP angle $\theta$ as counter-clockwise rotation starting at the positive x-axis and orient the polarizer so that it transmits horizontally polarized light. By measuring the power transmitted through the polarizer as a function of $\theta$, the four Stokes parameters can be determined by fitting the transmitted power data $I(\theta)$ with the following equation:

$$\begin{aligned} I(\theta) = \frac{1}{4}(2S_0 + S_1 + S_1\cos\eta) + \frac{1}{4}(S_1 + S_1\cos\eta)\cos(4\theta) \\ - \frac{1}{2}S_3\sin\eta\sin(2\theta) + \frac{1}{4}(S_2 - S_2\cos\eta)\sin(4\theta). \end{aligned}$$

where $\eta$ is the actual wavelength-dependent retardance of the QWP as provided by the manufacturer (Thorlabs AQWP10M-980). The different phases and frequency in $\theta$ allow for one measurement to fit all four Stokes parameters simultaneously.

The NIR laser polarization state was measured by placing the QWP and polarizer at the beam waist and using a standard optical power meter to measure the intensity as a function of QWP rotation angle, see Fig. S4(c). The sideband polarization states were measured in parallel using the EMCCD spectrometer to monitor the intensity of individual sidebands. The accuracy of this broadband polarimeter was tested by placing a rotatable polarizer at the sample position to provide a known polarization state, and shining collimated light from a tungsten-halogen lamp through the beam path. The polarization state as a function wavelength was able to predict the $\alpha$ of the test polarizer to within $1^\circ$.

One of the potential sources of systematic error in the polarization measurements comes from the alignment of the fast axis of the QWP. It was aligned by trying to align the fast axis with one of two crossed polarizers, and extinguishing the transmitted light. Any misalignment in the QWP directly results in an equivalent shift in the $\alpha$ angle of all of

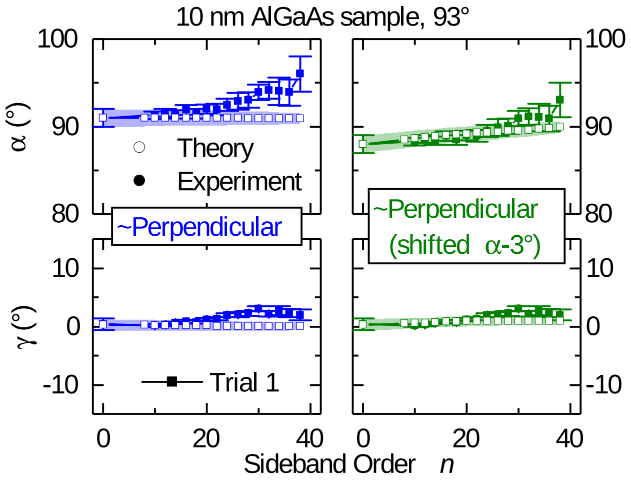


FIG. S3: (Left side) Directly reproduced from Fig. 5 of the main paper, but without the nearly parallel data of trial 2. (Right side) Same data set assuming a 3° offset in the QWP. The experimental data is shifted downward 3°, and the theory has been recalculated.

the data, but since the optics were realigned before each polarimetry trial due to space constraints in the experiment, the shift may only affect one trial.

To test if this misalignment could explain the disagreement between experiment and theory, let us assume the QWP was misaligned by 3°, and shift the experimental data and recalculate the expected polarization state for trial 1 of perpendicular, shown in Fig. S3. Just this small offset removes the deviation from experiment and theory for $\alpha$ for $n > 20$, and both experiment and theory agree within the error bars until the last order. This significant change for such a small offset indicates a very high degree of precision is needed for a quantitative comparison between theory and experiment, which is outside the scope of this work.

Similar to the polarization state measurements for the 10 nm AlGaAs sample, presented in Fig. 6 in the paper, measurements for the 10 nm GaAs sample were taken. The data sets from the two samples agree that the sideband polarization states depend very sensitively on the NIR laser polarization state. While the scale of the polarization angles is consistent between the experimentally measured and theoretically calculated polarization states, the trends are not well reproduced. Furthermore, using the polarization state data to measure the ratio $I_\perp/I_\parallel$ gets the trend correct that the ratio increases with increasing sideband order, but the scales do not agree. Thus a more careful experimental investigation of the sideband

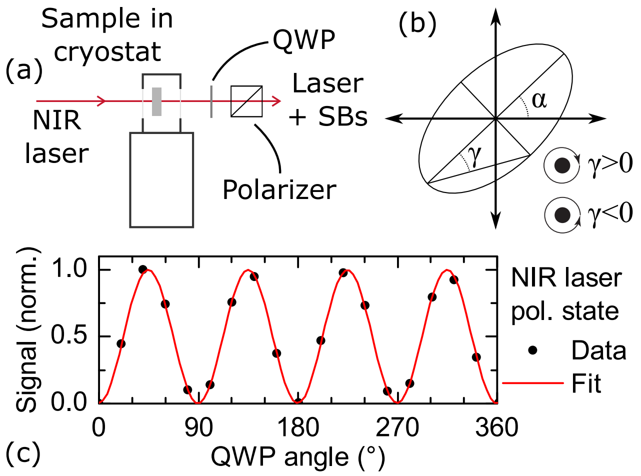


FIG. S4: Polarization state measurement details. (a) A quarter-wave plate (QWP) followed by a prism polarizer comprise the Stokes polarimeter, which is placed immediately after the cryostat to minimize the number of confounding optics. (b) Defining the angles of the polarization ellipse for a laser beam. The beam is propagating into the page. (c) The results of a Stokes polarimeter measurement of the NIR laser after transmitting through the sample. For this measurement $\alpha = -89.2 \pm 1°$ and $\gamma = 0.4 \pm 1°$.

polarization state, including the inconsistencies noted here, are outside the scope of the current paper.

## TERAHERTZ POLARIZATION MEASUREMENT

The polarization of the THz beam was also measured to ensure the driving field was linearly polarized. Wave retarders in the THz range are not as straightforward as in the optical regime and a full measurement of the polarization state was not possible. Instead, a rotating wire grid polarizer was placed at a beam waist in front of a horn-coupled pyroelectric detector (see Fig. SS6(a)). In this setup, the first three Stokes parameters can be measured. With the analyzer angle given by $\theta$, the power on the detector, $I(\theta)$ is now given by,

$$I(\theta) = \frac{S_0}{2} + \frac{S_1}{2}\cos(2\theta) + \frac{S_2}{2}\sin(2\theta)$$

From the fit of the measured intensity profile (Fig. S5(b)), the angle $\alpha$ can be backed

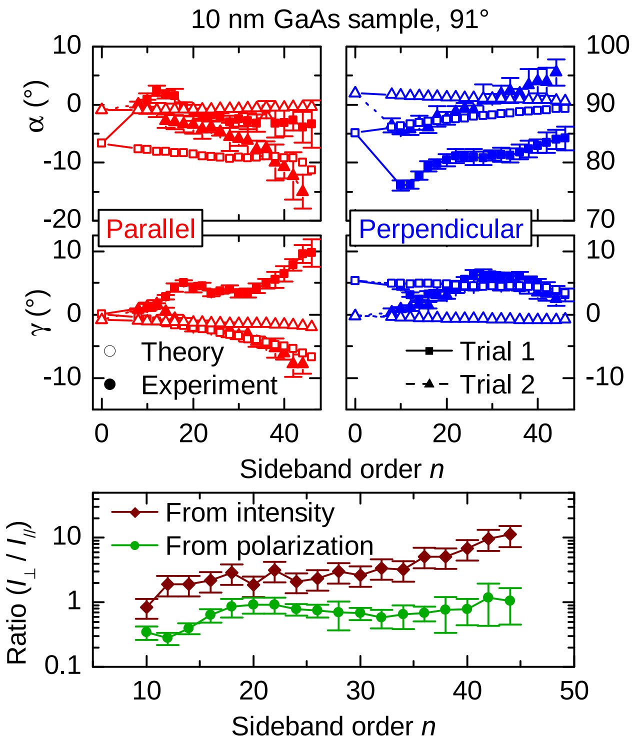


FIG. S5: Polarization state of the sidebands in terms of the two ellipticity angles from the 10 nm GaAs sample. (top) Experimental and theoretical values for the polarization angles. Experimental measurements are filled scatter points, theoretical calculations are empty scatter points. Polarization state measurements were performed for both excitation geometries, and all the measurements were duplicated with approximately the same NIR laser polarization. The NIR laser polarization state is plotted as the order zero sideband and circled in black for each measurement. Overall, both theory and experiment agree that the polarization state of a given sideband is extremely sensitive to the NIR laser polarization state. (bottom) Ratio of the different polarization geometries $I_\perp/I_\parallel$ from two independent measurements. The ratio is calculated from the intensity measurements, dark red diamond scatter points, and from the polarization state measurements from above, green circle scatter points.

out, as well as a "degree of linear polarization", $p_l$, which we define as,

$$p_l = \frac{\sqrt{S_1^2 + S_2^2}}{S_0}$$

Since this setup does not measure the third final component of the Stokes parameters, it is not possible to distinguish elliptically polarized light from unpolarized light. Thus, instead of a true degree of polarization, we can only calculate what fraction is linearly polarized.

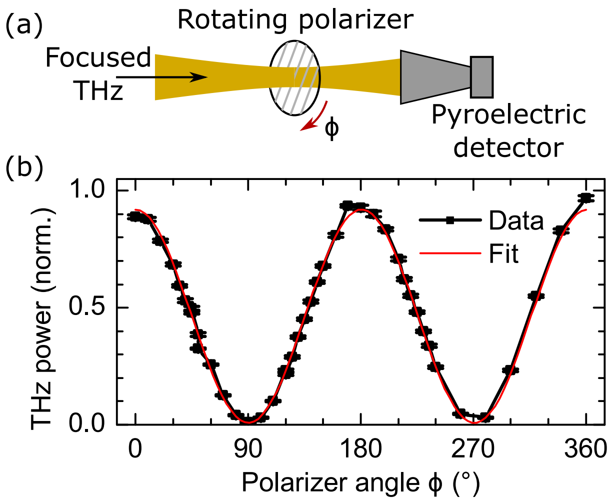


FIG. S6: Measuring THz polarization. (a) A wire grid polarizer is mounted to a rotatable stage and placed at the focus of the THz beam. A fast, horn-coupled pyroelectric detector is placed immediately behind the wire grid. (b) The THz power measured behind the polarizer as it was rotated. The signal was normalized the the signal when the polarizer was removed.

From the fit, the THz is polarized at $\alpha = 0.4 \pm 0.5°$, so almost perfectly horizontal in the lab frame, and it is 98.7±1.2% linearly polarized. The contrast ratio is likely limited by wire grid quality in either the linear polarimeter or the attenuator.

[1] D. Gammon, B. V. Shanabrook, and D. S. Katzer, Physical Review Letters **67**, 1547 (1991), URL `http://journals.aps.org/prl/abstract/10.1103/PhysRevLett.67.1547`.

[2] D. S. Katzer, D. Gammon, and B. V. Shanabrook, Journal of Vacuum Science & Technology B: Microelectronics and Nanometer Structures **10**, 800 (1991), ISSN 0734211X, URL `http://scitation.aip.org/content/avs/journal/jvstb/10/2/10.1116/1.586119`.

[3] R. F. Kopf, E. F. Schubert, T. D. Harris, and R. S. Becker, Applied Physics Letters **58**, 631 (1991), ISSN 00036951, URL `http://scitation.aip.org/content/aip/journal/apl/58/6/10.1063/1.104551`.

[4] M. A. Herman, D. Bimberg, and J. Christen, Journal of Applied Physics **70** (1991), ISSN 00218979.

[5] G. D. Cole, W. Zhang, M. J. Martin, J. Ye, and M. Aspelmeyer, Nat Photon **7**, 644 (2013),

ISSN 1749-4885, article, URL http://dx.doi.org/10.1038/nphoton.2013.174.

[6] G. D. Cole, W. Zhang, B. J. Bjork, D. Follman, P. Heu, C. Deutsch, L. Sonderhouse, J. Robinson, C. Franz, A. Alexandrovski, et al., Optica **3**, 647 (2016), URL http://www.osapublishing.org/optica/abstract.cfm?URI=optica-3-6-647.

[7] E. Yablonovitch, T. Gmitter, J. P. Harbison, and R. Bhat, Applied Physics Letters **51**, 2222 (1987), ISSN 00036951.

[8] E. Yablonovitch, D. M. Hwang, T. J. Gmitter, L. T. Florez, and J. P. Harbison, Applied Physics Letters **56**, 2419 (1990), ISSN 00036951.

[9] N. Q. Vinh, S. J. Allen, and K. W. Plaxco, Journal of the American Chemical Society **133**, 8942 (2011), ISSN 00027863.

[10] M. L. P. Bailey, A. T. Pierce, A. J. Simon, D. T. Edwards, G. J. Ramian, N. I. Agladze, and M. S. Sherwin, IEEE Transactions on Terahertz Science and Technology **5**, 961 (2015).

[11] J. R. Danielson, Y.-S. S. Lee, J. P. Prineas, J. T. Steiner, M. Kira, and S. W. Koch, Physical Review Letters **99**, 237401 (2007), ISSN 0031-9007, URL http://link.aps.org/doi/10.1103/PhysRevLett.99.237401.

[12] G. Ramian, Nuclear Instruments and Methods in Physics Research Section A: Accelerators, Spectrometers, Detectors and Associated Equipment **318**, 225 (1992), ISSN 01689002, URL http://www.sciencedirect.com/science/article/pii/016890029291056F.

[13] D. H. Goldstein, *Polarized Light* (Taylor and Francis Group, Boca Raton, FL, 2011), 3rd ed., ISBN 978-1-4398-3041-3.
