# Supplementary material for: Dynamical birefringence: Electron-hole recollisions as probes of Berry curvature
Source: arXiv:1706.08449 ancillary file (2017-10-12)
Supplement: Supplementary file 3 [file SI_J_Matrix.pdf]

# Electron-hole recollisions as probes of Berry curvature
# Supplementary: J Matrix

Qile Wu

September 13, 2017

For each order of sideband, we assign a Jones matrix [1] $\mathcal{J}_N$, which is defined as

$$\begin{bmatrix} E_{x,N,HSG} \\ E_{y,N,HSG} \end{bmatrix} = \mathcal{J}_N \begin{bmatrix} E_{x,NIR} \\ E_{y,NIR} \end{bmatrix}, \mathcal{J}_N = \begin{bmatrix} J_{N,xx} & J_{N,xy} \\ J_{N,yx} & J_{N,yy} \end{bmatrix}. \quad (1)$$

Following the input of NIR field described by Jones vector $[E_{x,NIR}, E_{y,NIR}]^T$, and an optical element, the THz driven quantum well, the produced HSG is given by the Jones vector $[E_{x,N,HSG}, E_{y,N,HSG}]^T$. The THz field is linearly polarized along the x-axis.

The experiment measures three quantities from each sideband with a fixed lattice orientation: the sideband efficiency $P_{measured,N}$ with intensity measured behind a polarizer picking out the component along the THz field, and the polarization angles $\alpha_N$, $\gamma_N$ (Fig. 1). From the polarization angles, we can determine the Jones vector for each sideband to within an unknown phase factor $e^{i\delta_N}$:

$$\begin{bmatrix} E_{x,N,HSG} \\ E_{y,N,HSG} \end{bmatrix} = \begin{bmatrix} |E_{x,N}| \\ |E_{y,N}|e^{i\Theta_N} \end{bmatrix} e^{i\delta_N}. \quad (2)$$

The $N$th order sideband, as a time-dependent monochromatic field, can be written as

$$\begin{bmatrix} |E_{x,N}| \\ |E_{y,N}|e^{i\Theta_N} \end{bmatrix} e^{i(\Omega t+N\omega t+\delta_N)} = \begin{bmatrix} \cos\alpha_N & -\sin\alpha_N \\ \sin\alpha_N & \cos\alpha_N \end{bmatrix} \begin{bmatrix} |E_{\|,N}|\cos\gamma_N \\ i|E_{\|,N}|\sin\gamma_N \end{bmatrix} e^{i(\Omega t+N\omega t+\delta'_N)}. \quad (3)$$

Similarly, the input NIR Jones vector is written as

$$\begin{bmatrix} E_{x,NIR} \\ E_{y,NIR} \end{bmatrix} = \begin{bmatrix} |E_{x,0}| \\ |E_{y,0}|e^{i\Theta_0} \end{bmatrix} e^{i\delta_0}, \quad (4)$$

with the complete time-dependent form

$$\begin{bmatrix} |E_{x,0}| \\ |E_{y,0}|e^{i\Theta_0} \end{bmatrix} e^{i(\Omega t+\delta_0)} = \begin{bmatrix} \cos\alpha_0 & -\sin\alpha_0 \\ \sin\alpha_0 & \cos\alpha_0 \end{bmatrix} \begin{bmatrix} |E_{\|,0}|\cos\gamma_0 \\ i|E_{\|,0}|\sin\gamma_0 \end{bmatrix} e^{i(\Omega t+\delta'_0)}, \quad (5)$$

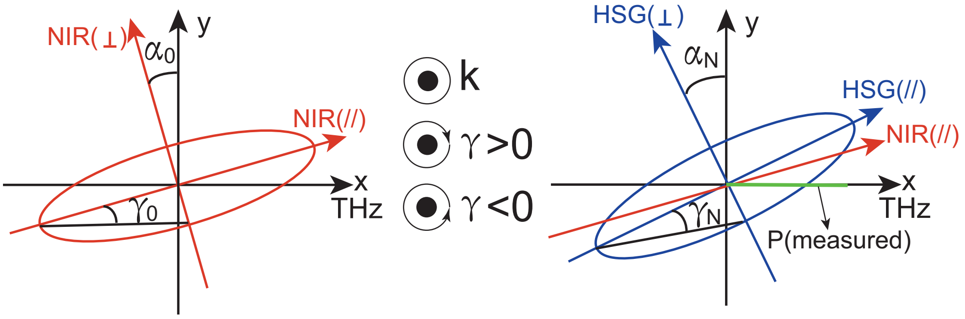


Figure 1: The measured quantities. NIR(∥) and NIR(⊥) indicates the major and minor axes of the NIR field, while HSG(∥) and HSG(⊥) are for the sideband. The NIR field and sideband emissions all propagate inwards. The angles $\gamma_0$ and $\gamma_N$ are defined to be positive when the electric field, observed from the source, rotates clockwise along the wave vector **k**. The green line indicates the polarization direction selected in the sideband efficiency measurement.

where $\delta_0$ is also an unknown phase.

Define

$$u_{x,N}e^{iv_{x,N}} = \cos\alpha_N \cos\gamma_N - i\sin\alpha_N \sin\gamma_N, \tag{6}$$

$$u_{y,N}e^{iv_{y,N}} = \sin\alpha_N \cos\gamma_N + i\cos\alpha_N \sin\gamma_N. \tag{7}$$

From each measurement of the polarization angles, we can obtain an equation for the Jones matrix elements by eliminating the unknown phases:

$$\frac{u_{x,0}e^{iv_{x,0}}J_{N,xx} + u_{y,0}e^{iv_{y,0}}J_{N,xy}}{u_{x,0}e^{iv_{x,0}}J_{N,yx} + u_{y,0}e^{iv_{y,0}}J_{N,yy}} = \frac{u_{x,N}e^{iv_{x,N}}}{u_{y,N}e^{iv_{y,N}}}, \tag{8}$$

or, in a linear form,

$$J_{N,xx} + \frac{u_{y,0}e^{iv_{y,0}}}{u_{x,0}e^{iv_{x,0}}}J_{N,xy} = (J_{N,yx} + \frac{u_{y,0}e^{iv_{y,0}}}{u_{x,0}e^{iv_{x,0}}}J_{N,yy})\frac{u_{x,N}e^{iv_{x,N}}}{u_{y,N}e^{iv_{y,N}}}. \tag{9}$$

We can solve $\frac{J_{N,xy}}{J_{N,xx}}, \frac{J_{N,yx}}{J_{N,xx}}, \frac{J_{N,yy}}{J_{N,xx}}$, from three different groups of polarization angles. If more than three groups of data exist, we can use an optimization procedure. For linear equations of the form $\sum_j A_{ij}x_j = b_i$, the idea is to minimize the function $f(x_1, x_2, ...) = \sum_i |\sum_j A_{ij}x_j - b_i|^2$. Let $\frac{\partial f}{\partial x_j^*} = 0$, then we obtain a new group of equations with a unique solution

$$\sum_k (\sum_i A_{ji}^\dagger A_{ik})x_k = \sum_i A_{ji}^\dagger b_i. \tag{10}$$

To determine the value of $J_{N,xx}$, we can use the equation

$$\frac{|E_{\|,N}|}{|E_{\|,0}|}u_{x,N}e^{i(v_{x,N}+\delta'_N)} = J_{N,xx}(u_{x,0}e^{iv_{x,0}} + u_{y,0}e^{iv_{y,0}}\frac{J_{N,xy}}{J_{N,xx}})e^{i\delta'_0}, \tag{11}$$

where $\frac{|E_{\|,N}|}{|E_{\|,0}|}$ can be deduced from the measured sideband efficiency, which can be written as

$$P_{measured,N} = \frac{|E_{\|,N}|^2}{|E_{\|,0}|^2}[u_{x,N}^2 \cos^2 \alpha_N + u_{y,N}^2 \sin^2 \alpha_N + u_{x,N} u_{y,N} \sin(2\alpha_N) \cos(v_{x,N} - v_{y,N})], \tag{12}$$

We can see that, the absolute value of $J_{N,xx}$ can be obtained but the determination of its phase requires the knowledge of the relative phase of NIR and sideband emission. Note here that if the dephasing rate is a constant, $\frac{J_{N,xy}}{J_{N,xx}}, \frac{J_{N,yx}}{J_{N,xx}}, \frac{J_{N,yy}}{J_{N,xx}}$ will be independent of dephasing, which is not true for $J_{N,xx}$.

In conclusion, the Jones matrix $\mathcal{J}_N$ can be determined to within an unknown phase factor from the measured sideband efficiency and the polarization angles of the sideband. If the relative phase of the NIR field and the sideband emission is measured, the Jones matrix can be completely determined.

Using the Jones matrix, one can estimate the error in sideband polarization propagated from the error in NIR laser polarization. Consider the case for low positive order sidebands ($n \leq 40$) where the dynamical Jones matrix $\mathcal{J}_N$ is approximately diagonal, and $J_{N,xx}/J_{N,yy}$ is approximately real. In this case, we have

$$\begin{bmatrix} E_{x,N,HSG} \\ E_{y,N,HSG} \end{bmatrix} = \begin{bmatrix} J_{N,xx} E_{x,NIR} \\ J_{N,yy} E_{y,NIR} \end{bmatrix}, \tag{13}$$

where

$$\begin{bmatrix} E_{x,N,HSG} \\ E_{y,N,HSG} \end{bmatrix} = \begin{bmatrix} \cos\alpha_N & -\sin\alpha_N \\ \sin\alpha_N & \cos\alpha_N \end{bmatrix} \begin{bmatrix} |E_{\|,N}| \cos\gamma_N \\ i|E_{\|,N}| \sin\gamma_N \end{bmatrix} e^{i\delta_N}, \tag{14}$$

$$\begin{bmatrix} E_{x,NIR} \\ E_{y,NIR} \end{bmatrix} = \begin{bmatrix} \cos\alpha_0 & -\sin\alpha_0 \\ \sin\alpha_0 & \cos\alpha_0 \end{bmatrix} \begin{bmatrix} |E_{\|,0}| \cos\gamma_0 \\ i|E_{\|,0}| \sin\gamma_0 \end{bmatrix} e^{i\delta_0}. \tag{15}$$

For $\alpha_0 \approx 0$ and $\gamma_0 \approx 0$, we have $\alpha_N \approx 0$ and $\gamma_N \approx 0$. Expanding Eq. 13 to the first order of the polarization angles, we obtain

$$\begin{bmatrix} 1 \\ \alpha_N + i\gamma_N \end{bmatrix} = \frac{|E_{\|,0}|}{|E_{\|,N}|} \begin{bmatrix} J_{N,xx} \\ J_{N,yy}(\alpha_0 + i\gamma_0) \end{bmatrix} e^{i(\delta_0 - \delta_N)}. \tag{16}$$

Thus the errors in the polarization angles of the NIR laser $\delta\alpha_0$ and $\delta\gamma_0$ induces errors in the sideband polarizations as

$$\delta\alpha_N^{\|} = \frac{J_{N,yy}}{J_{N,xx}} \delta\alpha_0, \tag{17}$$

and

$$\delta\gamma_N^{\|} = \frac{J_{N,yy}}{J_{N,xx}} \delta\gamma_0. \tag{18}$$

Similarly, for $\alpha_0 \approx \pi/2$ and $\gamma_0 \approx 0$, we have $\alpha_N \approx \pi/2$ and $\gamma_N \approx 0$, and

$$\begin{bmatrix} \alpha_N - \pi/2 - i\gamma_N \\ 1 \end{bmatrix} \approx \frac{|E_{\|,0}|}{|E_{\|,N}|} \begin{bmatrix} J_{N,xx}(\alpha_0 - \pi/2 - i\gamma_0) \\ J_{N,yy} \end{bmatrix} e^{i(\delta_0 - \delta_N)}, \quad (19)$$

from which we can get the errors

$$\delta\alpha_N^{\perp} = \frac{J_{N,xx}}{J_{N,yy}} \delta\alpha_0, \quad (20)$$

and

$$\delta\gamma_N^{\perp} = \frac{J_{N,xx}}{J_{N,yy}} \delta\gamma_0. \quad (21)$$

We can see that the errors for the nearly parallel case and the nearly perpendicular case are different, with a ratio

$$|\frac{\delta\alpha_N^{\perp}}{\delta\alpha_N^{\|}}| = |\frac{\delta\gamma_N^{\perp}}{\delta\gamma_N^{\|}}| = |\frac{J_{N,xx}}{J_{N,yy}}|^2. \quad (22)$$

Interestingly, this ratio is just the sideband intensity ratio.

# References

[1] R Clark Jones. A new calculus for the treatment of optical systems I. Description and discussion of the calculus. *J. Opt. Soc. Am.*, 31(7):488–493, 1941.
