# Supplementary material for: Dynamical birefringence: Electron-hole recollisions as probes of Berry curvature
Source: arXiv:1706.08449 ancillary file (2017-10-12)
Supplement: Supplementary file 4 [file SI_Quantum_Simulation.pdf]

# Electron-hole recollisions as probes of Berry curvature
# Supplementary: Quantum Simulation

Qile Wu

September 13, 2017

To calculate the polarization vector

$$\vec{\mathbb{P}}(t)=\frac{1}{V}\sum_{s,\mathbf{k}}\vec{\mu}_s U_s^{\dagger}[\mathbf{k}(t)]\eta_{\mathbf{k}(t),s}(t)+c.c., \tag{1}$$

we numerically solve the Heisenberg equation

$$i\hbar\frac{d\eta_{\mathbf{k}(t),s}}{dt}=\Lambda[\mathbf{k}(t)]\eta_{\mathbf{k}(t),s}-e\mathbf{E}_{THz}(t)\cdot\vec{R}_s[\mathbf{k}(t)]\eta_{\mathbf{k}(t),s}-U_s[\mathbf{k}(t)]\vec{\mu}_s\cdot\mathbf{E}_{NIR}(t)-i\hbar\gamma_{2,s}[\mathbf{k}(t)]\eta_{\mathbf{k}(t),s}. \tag{2}$$

Firstly, since it is a linear differential equation, we can solve the equation with delta sources and then do a summation. Secondly, the photon energy of the NIR field can be subtracted from the energy levels before finite difference calculation so as to make the algorithm achieve stability more easily. In other words, we shall instead solve the equation:

$$i\hbar\frac{d\bar{\eta}_{\mathbf{k}(t),s,t_0}}{dt}=\bar{\Lambda}[\mathbf{k}(t)]\bar{\eta}_{\mathbf{k}(t),s,t_0}-e\mathbf{E}_{THz}(t)\cdot\vec{R}_s[\mathbf{k}(t)]\bar{\eta}_{\mathbf{k}(t),s,t_0}-i\hbar\gamma_{2,s}[\mathbf{k}(t)]\bar{\eta}_{\mathbf{k}(t),s,t_0}, \tag{3}$$

with initial condition $\bar{\eta}_{\mathbf{k}(t),s,t_0}|_{t=t_0}=-\frac{\Delta t_0}{\hbar}U_s[\mathbf{k}(t_0)]\vec{\mu}_s\cdot\mathbf{F}_{NIR}$, where, $\bar{\Lambda}=\Lambda-\hbar\Omega$, and $\eta_{\mathbf{k}(t),s}=e^{-i\Omega t}\sum_{t_0}\bar{\eta}_{\mathbf{k}(t),s,t_0}$, $t_0\in(-\infty,t]$.

Set $\bar{\eta}_{\mathbf{k}(t),s,t_0}=e^{-\frac{i}{\hbar}\int_{t_0}^{t}dt''\bar{\Lambda}[\mathbf{k}(t'')]}\xi_{\mathbf{k}(t),s,t_0}$ to eliminate the energy term, and we have

$$i\hbar\frac{d}{dt}\xi_{\mathbf{k}(t),s,t_0}=-e\mathbf{E}_{THz}\cdot e^{\frac{i}{\hbar}\int_{t_0}^{t}dt''\Lambda[\mathbf{k}(t'')]}\vec{R}_s[\mathbf{k}(t)]e^{-\frac{i}{\hbar}\int_{t_0}^{t}dt''\Lambda[\mathbf{k}(t'')]}\xi_{\mathbf{k}(t),s,t_0}-i\hbar\gamma_{2,s}(\mathbf{k})\xi_{\mathbf{k}(t),s,t_0}, \tag{4}$$

or, for the nth subband component

$$i\hbar\frac{d}{dt}\xi_n=-e\mathbf{E}_{THz}\cdot\sum_m\langle v_n(\mathbf{k})|i\partial_{\mathbf{k}}v_m(\mathbf{k})\rangle e^{-\frac{i}{\hbar}\int_{t_0}^{t}dt''[E_m(\mathbf{k}(t''))-E_n(\mathbf{k}(t''))]}\xi_m-i\hbar\gamma_{2,n}(\mathbf{k})\xi_n, \tag{5}$$

with initial condition $\xi_{\mathbf{k}(t),s,t_0}|_{t=t_0} = -\frac{\Delta t_0}{\hbar} U_s[\mathbf{k}(t_0)]\vec{\mu}_s \cdot \mathbf{F}_{NIR}$. We combine the leap-frog method and Crank-Nicolson method to cope with the dephasing term:

$$\xi_n(\Delta t) = (1-\gamma_{2,n}[\mathbf{k}(0)]\Delta t)\xi_n(0) - \frac{\Delta t}{i\hbar} e\mathbf{E}_{THz}(0) \cdot \sum_m \langle v_n(\mathbf{k})|i\partial_{\mathbf{k}}|v_m(\mathbf{k})\rangle|_{\mathbf{k}(0)}\xi_m(0), \tag{6}$$

$$\xi_n(t+\Delta t) = (1+\gamma_{2,n}[\mathbf{k}(t)]\Delta t)^{-1}[-\frac{2\Delta t}{i\hbar} e\mathbf{E}_{THz}(t) \cdot \sum_m \langle v_n(\mathbf{k})|i\partial_{\mathbf{k}}|v_m(\mathbf{k})\rangle|_{\mathbf{k}(t)}$$
$$\cdot e^{-\frac{i}{\hbar}\int_{t_0-\tau}^{t} dt''[E_m(\mathbf{k}(t''))-E_n(\mathbf{k}(t''))]}\xi_m(t) + (1-\gamma_{2,n}[\mathbf{k}(t)]\Delta t)\xi_n(t-\Delta t)]. \tag{7}$$

To calculate the Berry connection, a gauge smoothing procedure is needed. We fix the gauge at $\mathbf{k} = \mathbf{0}$, where we take the cellular functions as $f_n|u_j\rangle$. For the gauge at a nonzero $\mathbf{k}_0$, we project each cellular function $f_n|u_j\rangle$ along the k-space straight line connecting $\mathbf{0}$ and $\mathbf{k}_0$, step-by-step as

$$|v_n(\mathbf{k}+\Delta\mathbf{k})\rangle = N_v W_j(\mathbf{k}+\Delta\mathbf{k}) W_j^\dagger(\mathbf{k}+\Delta\mathbf{k})|v_n(\mathbf{k})\rangle, \tag{8}$$

where $N_v$ is a normalization constant. This formula is gauge invariant, avoiding random phases of the wave functions from numerical calculation, and $W_j(\mathbf{k}) = (|w_{j,1}(\mathbf{k})\rangle, |w_{j,2}(\mathbf{k})\rangle, ..., |w_{j,g}(\mathbf{k})\rangle)$ is a othonormal basis of the jth subband from numerical calculation. For our system, each subband is doubly degenerate, so $g = 2$. Alternatively, in our band model, the subbands can also be divided into two groups by hand, $E_{1,\downarrow}, HH_{1,\uparrow}, HH_{2,\downarrow}$ for one group, and $E_{1,\uparrow}, HH_{1,\downarrow}, HH_{2,\uparrow}$ for the other. In either group, we have $g = 1$ for each subband.

To calculate the polarization vector $\vec{\mathbb{P}}(t)$, we still need to determine the relevant k-points, the range of time $t$ for Fourier transformation, the range of initial time $t_0$ and the time step $\Delta t_0$ .

# 1 Relevant k-points

At first, we have an estimation of the relevant electron-hole pairs created by the pumping NIR field through the formula $\frac{|p_{cv}|^2}{\Delta^2+\gamma_2^2}$. The NIR frequency is resonant with the energy gap of the quantum well, and the dephasing rate is taken to be a constant $\gamma_2 = 1meV$. The NIR field is polarized as $\sigma^-_{NIR} = \frac{\hat{X}+i\hat{Y}}{2}$ or $f_1|\frac{3}{2}, +\frac{3}{2}\rangle$ component, and $\sigma^+_{NIR} = -\frac{\hat{X}-i\hat{Y}}{2}$ for $f_1|\frac{3}{2}, -\frac{1}{2}\rangle(\hat{X}, \hat{Y}$ are unit vectors along [010] and [001] respectively.). So $|p_{cv}|^2 = |d|^2|\alpha(\mathbf{k})|^2$, where, $d = \langle S|x|X\rangle$ is the dipole matrix element, and $\alpha(\mathbf{k})$ is the coefficient of the component $f_1|\frac{3}{2}, +\frac{3}{2}\rangle$ or $f_1|\frac{3}{2}, -\frac{1}{2}\rangle$ in the cellular function. Fig. 1 shows $\frac{|\alpha(\mathbf{k})|^2}{\Delta^2+\gamma_2^2}$ as a function of $\mathbf{k}$ along [100] for the components $f_1|\frac{3}{2}, +\frac{3}{2}\rangle, f_1|\frac{3}{2}, -\frac{1}{2}\rangle$ in HH1 and HH2 subbands. It can be seen that the resonant excitation is dominant. So we only consider the electron-hole pair created at $\mathbf{k}(t_0) = \mathbf{0}$.

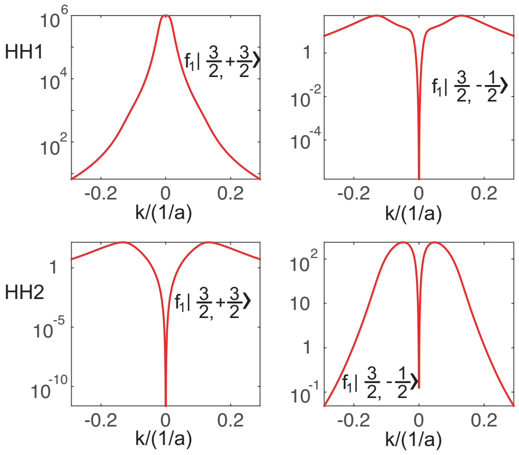


Figure 1: Estimation excitation strength for the 5nm quantum well. The first row is for HH1 band, and the second row is for HH2 band. The first column is for the heavy hole component $f_1|\frac{3}{2},+\frac{3}{2}\rangle$ and the second column is for the light hole component $f_1|\frac{3}{2},-\frac{1}{2}\rangle$.

| | $\hbar\gamma_p/meV$ | $\hbar\gamma_e/meV$ |
|---|---|---|
| 5nm GaAs | 2 | 2 |
| 10nm GaAs | 0.65 | 0.65 |
| 10nm AlGaAs | 2.25 | 2.25 |

Table 1: Parameters $\hbar\gamma_p$ and $\hbar\gamma_e$.

Next, we determine the critical k-points beyond which the electron or hole will reach the barrier region and be neglected. For example, as shown in Fig. 2, the subbands of the 5nm GaAs quantum well along [010] are plotted. The THz field is also linearly polarized along [010]. The energy levels are limited within the well region. The critical k-points in this case are $k_{cri} = \pm 0.2908a^{-1}$.

Then we partition the subbands into regions with different numbers of constant energy circles(Fig. 2), and model the dephasing rate as

$$\hbar\gamma_{2,s,n}(\mathbf{k}) = \hbar\gamma_p + [G_{n,c}(\mathbf{k}) + G_{n,v}(\mathbf{k})]\hbar\gamma_e, \tag{9}$$

where $n$ is the band index, and $G_{n,c}(\mathbf{k})(G_{n,v}(\mathbf{k}))$ is the number of constant energy circles for the electron(hole) to be scattered when the relative momentum of the electron-hole pair is $\hbar\mathbf{k}$. The parameters $\hbar\gamma_p$ and $\hbar\gamma_e$ used in the calculation are listed in Table. 1.

The last thing about $\mathbf{k}$ is that before the finite difference calculation, we calculate the Berry connection and energy levels in $[-k_{cri}, +k_{cri}]$ with spacing $\Delta k = 0.001k_{cri}$.

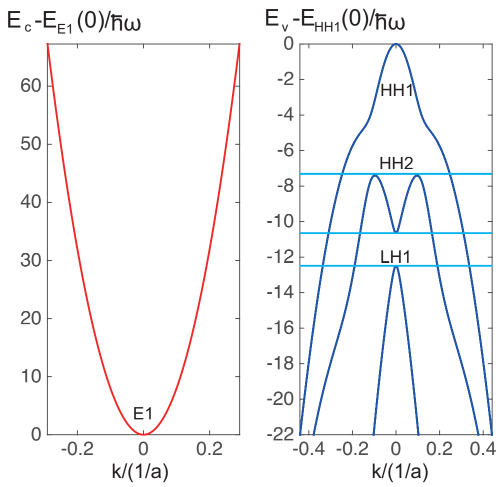


Figure 2: Band structure along [010] for the 5nm GaAs quantum well. $E_{E1}(0)$ and $E_{HH1}(0)$ are respectively the conduction band minimum and valence band maximum, which are taken as the energy references for the energy levels for the conduction subbands $E_c$ and valence subbands $E_v$. The energy of one THz photon $\hbar\omega$ is used as the unit of energy. The blue straight lines partition the subbands into regions with different numbers of elastic scattering channels.

## 2 Range of time $t$ for Fourier transformation

In higher-order sideband generation, indeed the polarization vector $\vec{\mathbb{P}}(t)$ as a whole is not a periodic function of time. However, if we factor out the frequency of the pumping NIR field, the polarization vector should have the same periodicity as the THz field. If no special representation is used, the polarization vector can be written as

$$\langle g|\vec{\mathbb{P}}(t)|g\rangle = \frac{i}{\hbar}\int_0^{+\infty} d\tau \int \frac{d\mathbf{P}}{(2\pi)^2}\langle g|e\mathbf{r}\hat{T}[e^{-\frac{i}{\hbar}\int_{t-\tau}^{t}\{\mathbf{H}[\mathbf{P}-\frac{e}{\hbar}\mathbf{A}(t'')]-\hbar\Omega\}dt''}]e\mathbf{r}|g\rangle\cdot\mathbf{F}_{NIR}e^{-i\Omega t}, \tag{10}$$

where $\mathbf{r}, \mathbf{H}$ are respectively the position operator, and the Hamiltonian operator describing the relative motion of the electron-hole pairs including the dephasing term. We have neglect the complex conjugate part involving the factor $e^{i\Omega t}$ because the frequency of the THz field is about three orders of magnitude lower than the one of the NIR field and the two frequencies are incommensurate in general. From the periodicity of the vector potential $\mathbf{A}(t)$ for the THz field, we can see that $\langle g|\vec{\mathbb{P}}(t)|g\rangle e^{i\Omega t}$ has the period of the THz field. For our special case, due to in-plane inversion symmetry of the GaAs quantum well, the period can be halved, which can be seen by

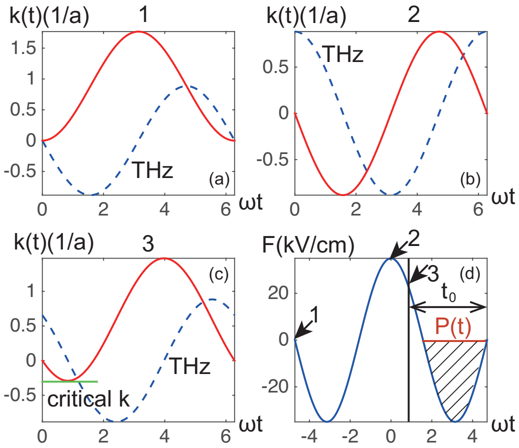


Figure 3: The range of $t$ and $t_0$ for 5nm GaAs quantum well. (a)(b)(c)The evolution of the kinetic momentum for three different initial time $t_0$ as indicated in (d). The dashed lines show the phase of the THz field. (d)The THz field strength as a function of time. The shaded region indicates the range of time $t$ for calculating the polarization vector.

transformation

$$\mathbf{H}[\mathbf{P}-\frac{e}{\hbar}\mathbf{A}(t)] \to \mathbf{H}[-\mathbf{P}-\frac{e}{\hbar}\mathbf{A}(t)] = \mathbf{H}[\mathbf{P}+\frac{e}{\hbar}\mathbf{A}(t)] = \mathbf{H}[\mathbf{P}-\frac{e}{\hbar}\mathbf{A}(t+\frac{\pi}{\omega})]. \quad (11)$$

Therefore, in order to get the sideband spectrum, we only need to calculate $\vec{\mathbb{P}}(t)$ in half the period of the THz field, As shown in the shaded region in Fig. 3(d). This also explains why only even orders of sideband are observed.

## 3 Range of initial time $t_0$

If there is no dephasing effect, in principle, we need to do the calculation for all $t_0 \in (-\infty, t]$ in order to get the polarization vector at $t$. However, the THz field in our problem is so strong that the electron-hole pairs are easy to be driven into the barrier region. In other words, as shown in Fig. 3(d), the electron-hole pair should be able to reach the shaded region in order to make contributions to the polarization vector. If the electron-hole pair is created when the initial strength of the THz field is zero(Fig. 3(a)), then within a half period of the THz field, the electron-hole pair will touch the barrier region. When the initial strength of the THz field is at the peak value, the electron-hole pair still cannot survive to get to the shaded region (Fig. 3(b)). Fig. 3(c) shows the first and also the longest $\mathbf{k}(t)$ trajectory involved in our calculation. When the electron-hole pair is created after the

time point #3(Fig. 3(d)), it can always get to the shaded region before the critical kinetic momentum is reached. So we have the range of $t_0$ shown in Fig. 3(d).

# 4 Time step $\Delta t_0$

The time step $\Delta t_0$ is related to the accuracy of the sideband spectrum and the stability of the finite difference calculation.

The sideband spectrum is obtained from the knowledge of the polarization within one THz period. 10 equidistant points can determine a sinusoidal function by Fourier transformation to an accuracy of about 98 percent. So when the maximum order of sideband is $N_{max}$, we have an upper bound for the time difference $\Delta t_0 \leq \frac{2\pi}{10 N_{max}\omega}$. The stability condition for the finite difference calculation is estimated as $\omega\Delta t_0 < \frac{\hbar\omega}{e|\mathbf{F}_{THz}|||R||}$, where $||R||$ is the norm of Berry connection matrix. So we have $\omega\Delta t_0 < \min\{\frac{\pi}{5N_{max}}, \frac{\hbar\omega}{e|\mathbf{F}_{THz}|||R||}\}$.
