# Supplementary material for: Dynamical birefringence: Electron-hole recollisions as probes of Berry curvature
Source: arXiv:1706.08449 ancillary file (2017-10-12)
Supplement: Supplementary file 5 [file SI_semiclassical_calculation.pdf]

# Electron-hole recollisions as probes of Berry curvature
# Supplementary: Semiclassical Calculation

Qile Wu

September 13, 2017

Here we are aiming at extracting a semiclassical solution that dominates the physics from the equations:

$$Re\{\frac{\mathbf{F}_{NIR}\cdot\mathbf{D}_s^\dagger(t')\Lambda_s[\mathbf{k}(t')]\phi_s(t')}{\mathbf{F}_{NIR}\cdot\mathbf{D}_s^\dagger(t')\phi_s(t')}\}=\hbar\Omega, \tag{1}$$

$$\hbar\dot{\mathbf{k}}=e\mathbf{F}_{THz}\cos(\omega t), \tag{2}$$

$$\int_{t'}^{t}\{\phi_s^\dagger(t'')\frac{1}{\hbar}[D_{\mathbf{k}}^s,\Lambda_s[\mathbf{k}(t'')]]\phi_s(t'')-\dot{\mathbf{k}}(t'')\times\phi_s^\dagger(t'')\vec{\mathbb{F}}[\mathbf{k}(t'')]\phi_s(t'')\}dt''=0, \tag{3}$$

$$i\hbar\frac{d\phi_s}{dt}=\Lambda_s[\mathbf{k}(t)]\phi_s-e\mathbf{E}_{THz}(t)\cdot\vec{R}_s[\mathbf{k}(t)]\phi_s, \tag{4}$$

$$Re\{\frac{\hat{E}_l\cdot\mathbf{D}_s^\dagger(t)\Lambda_s[\mathbf{k}(t)]\phi_s(t)}{\hat{E}_l\cdot\mathbf{D}_s^\dagger(t)\phi_s(t)}\}=\hbar(\Omega+N\omega). \tag{5}$$

For the creation of electron-hole pairs, we assume that the NIR field is resonant with the energy gap. The initial state is determined by the first equation, but we don't need to exactly solve it. An estimation of the optical excitation strength from the formula $\frac{|p_{cv}|^2}{\Delta^2+\gamma_2^2}$($p_{cv}$ is the interband dipole matrix element, and $\Delta,\gamma_2$ are the detuning and dephasing rate respectively.) indicates that the resonant excitations give the major contribution. (Refer to the supplementary material "quantum simulation".) Thus we set $\mathbf{k}(t')=\mathbf{0}$, and the initial spinor state $\phi_s(t')=(1,0)^T$ for both $s=\uparrow$ and $s=\downarrow$.

To completely determine the evolution of the spinors and the semiclassical trajectories, we need to know the initial phase $\varphi=\omega t'$ of the THz field when the electron-hole pairs are created. Given $\varphi$, from $\hbar\dot{\mathbf{k}}=e\mathbf{F}_{THz}\cos(\omega t)$, we have $\mathbf{k}(t)=\frac{e\mathbf{F}_{THz}}{\hbar}[\sin(\omega t)-\sin\varphi]$. The evolution of the pseudo-spin is calculated by finite difference method. Once $\mathbf{k}(t)$ and $\phi_s(t)$ are solved, the real space trajectories of the electron and hole can be determined. If the THz field is linearly polarized, as in our case, the trajectories of the kinetic

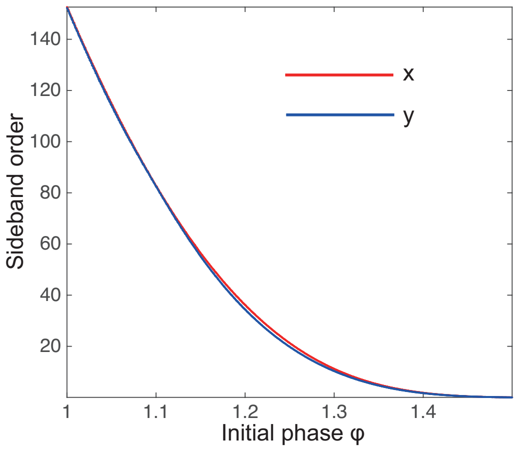


Figure 1: The correspondence between sideband order and the initial phase of the THz field in the 10 nm GaAs QWs. The red and blue curves are for $\hat{E}_l = \hat{x}([010])$ and $\hat{E}_l = \hat{y}([001])$ respectively.

momenta are collinear with the THz electric field. Not all such trajectories can end up with recollisions. The Lorentz-like velocity of the hole wavepackets induced by Berry curvature greatly increase the difficulty of exact recollisions. For simplicity, we ignore this velocity in the recollision condition.

For certain $\varphi$, at recollision, with $\mathbf{k}(t)$ and $\phi_s(t)$, the weighted average energy can be calculated and compared with the sideband photon energy. In this way, a correspondence between initial phase $\varphi$ and sideband order $N$ can be established. In our type-I QWs, the THz field is so strong that the electron or hole will always reach the barrier region within one half period of the THz field. In the barrier region, due to the existence of extended states, we expect large dephasing rates for the electron-hole pairs. So the electron-hole pairs stepping into the barrier region will be ignored. Under this assumption, for $\varphi \in (0, \frac{\pi}{2})$, $N$-$\varphi$ correspondence is one-to-one, as shown in Fig. **??**. Notice that for fixed sideband order, the initial phases are generally different for different HSG polarizations measured. Different initial phases imply different semiclassical trajectories. Fig. **??** shows the minor effect of this difference on the dynamical linear birefringence.

To simplify the construction of a semiclassical picture, we use the $N$-$\phi$ relation averaged for $\hat{E}_l = \hat{x}([010])$ and $\hat{E}_l = \hat{y}([001])$. With this, reversely, for a certain sideband order $N$, we can find a unique $\varphi$, which determines the k-space trajectory $\mathbf{k}(t)$, the evolution of the pseudo-spin $\phi_s(t)$, and the real space trajectory, so that a whole semiclassical picture can be established.

Now we can justify the neglect of the Lorentz-like velocity in the recollision condition. As shown in Fig. **??**, in the 10 nm GaAs QWs, for sidebands

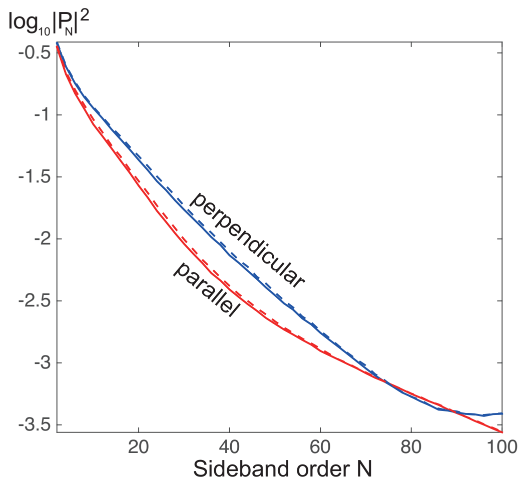


Figure 2: Sideband intensities for two configurations of the external fields in the 10 nm GaAs QWs. The THz field is linearly polarized along [010], while the polarization of the NIR field is rotated from [010](red curve) to [001](blue curve). The solid lines are calculated according to the average of the two $N$-$\phi$ relations in Fig. **??**, while the dashed lines are calculated with the $N$-$\phi$ relation for $\hat{E}_l = \hat{x}([010])$.

of orders less than 60, the deviation of the hole wave-packet center from the calculated recollision point lies within 10 lattice constants, and can reach beyond 45 lattice constants for the 100th order sideband.

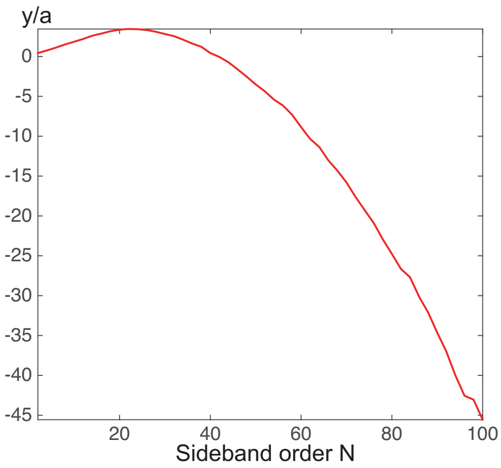


Figure 3: The component of the radius vector perpendicular to the THz field for the holes as a function of the sideband order in the 10 nm GaAs QWs. The THz field is linearly polarized along [010]. $a = 5.65\mathring{A}$ is the lattice constant of bulk GaAs.
